# Supplementary material for: ForceSight: Text-Guided Mobile Manipulation with Visual-Force Goals
Source: arXiv:2309.12312 source file (2023-09-24)
Supplement: Supplementary file 1 [file appendix.tex]

\section*{Appendix}
% \appendix
 % Change section numbering to alphabetical

% \youliang{All supplementary materials will be located here, we will break it into a different doc soon}

% \subsubsection*{A. Subgoal Transition}

% \begin{figure}[H]
%   \centering
%   % \vspace{2mm}
%   \includegraphics[width=.5\linewidth]{images/goals_diagram_1.png}
%   % \vspace{-2mm}
%   \caption{Venn diagram illustrates the start and end state of the robot overlaps when executing each subgoal. The overlaps transitional state is resolved by having action primitive added in the prompt. \cody{remove this, placeholder, maybe include}}
%   \label{fig:venn_diagram}
%    %\vspace{-15mm}
% \end{figure}

\section{Task Definition}
\label{appendix:task_def}

In our real-world experimentation, we evaluated 10 household tasks, each defined by sequences of action primitives. To determine the success rate for each task, we establish clear criteria for what constitutes a successful completion for each task and subtask.

We define success for each subtask by whether the kinematic and force errors meet criteria specified in the low-level controller \jeremy{add to main paper}, as is described in Appendix \ref{appendix:controller}.

For tasks that involve picking (e.g. \textit{``pick up the apple"}), the robot should successfully approach, grasp, and lift the target object above the surface for more than 5 seconds.

For placing tasks (e.g.\textit{ ``place the object in the hand"}), the robot should successfully approach the desired target object, ungrasp and place the held object to the target object. In this case, into a trash can or a static human hand.

For the \textit{``turn off the light switch"} task, the light switch should be completely toggled down to be considered a success.

Additionally, for \textit{``open the drawer"} task, the robot must successfully pull the drawer open, extending to its full range of motion. 

Finally, we label the execution of a task a failure if the trial does not terminate within a 1-minute time window. 

\section{Data Collection Setup}
\label{appendix:data-col-setup}

In order to collect visual data, we mount an Intel® RealSense™ D405 \cite{intelrealsenseDepthCamera} to the robot's gripper to capture the RGBD image $I$. The fingertips are first localized in the image via ArUco tags attached to the gripper, and a transformation is applied to map these to the point at the center of the fingertip surface, which we call the fingertip locations, denoted as $C_{LR} \in R^{2 \times 3}$ (left and right). Instead of using fiducial markers, this can be readily replaced with other detection methods, such as NN-based object detection. Subsequently, the 3D fingertip contact locations are then mapped from the future camera frame to the current frame by utilizing the robot's forward kinematics. We use a Stretch mobile manipulator for data collection. Certainly, this can also be substituted with different data collection setups as long as the ground truth future fingertip location can be obtained.

The force applied to the gripper is measured by a wrist-mounted force/torque sensor \cite{ATI}. This sensor provides accurate readings of the forces exerted by the gripper, enabling our system to predict future forces and enabling the robot to perform tasks requiring force control.

\label{desc:grasp-force-desc}
The grip force measurement is not natively available on the Stretch robot gripper. To obtain the grip force, we trained a small neural network, parameterized as an MLP, to estimate the grip force $F_G$ given the gripper motor state and fingertip positions. To provide ground truth for the grip force model, we grasp a force/torque sensor \cite{ATI} at various grip strengths and grasp widths and record the measured magnitude of the force.

\section{Data Collection details}

\label{appendix:data-collection}

We collect a dataset $D$, with $D_i = \{I,T,C_{LR},F_G, F_R\}$, where $I \in \mathbb{R}^{H \times W \times 4}$ is an RGBD image captured by a gripper-mounted camera, $T$ is a text prompt associated with a task and includes an action primitive, and $C_{LR} \in \mathbb{R}^{2 \times 3}$ is a set of two 3D fingertip locations in the camera frame associated with the next keyframe. Grip force $F_G$ and Applied force $F_A$ are described in Section \ref{sec:method}. These combined elements constitute the data points in the dataset, providing a comprehensive representation of a robot's interaction with its environment. From these datapoints, the kinematic and force goals ($G_K$ and $G_F$) that serve as ground truth for our network can be derived.

\begin{figure*}
  \centering
  % \vspace{2mm}
  \includegraphics[width=.8\linewidth]{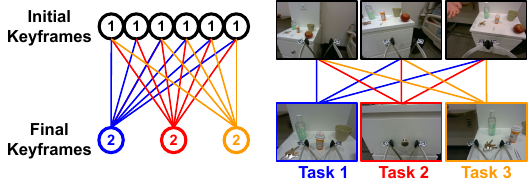}
  % \vspace{-2mm}
  \caption{\textbf{Left:} During data collection, we partition each task into pairs of hand-specified keyframes. During each data collection session, we pair keyframes associated with several initial gripper poses to a single final keyframe. \textbf{Right:} We are also able to pair these initial keyframes with final frames associated with additional tasks. \cody{add more detail, using the same frames for many different tasks}}
  \label{fig:data-collection2}
   \vspace{-5mm}
\end{figure*}

To collect training data for our system, an expert human operator controls the robot using a keyboard in order to capture RGBD images, text prompts, action primitives, and their corresponding visual-force goals. The kinematic goals and force goals that comprise a visual-force goal are mapped from the future camera frame to the current frame by utilizing the robot's forward kinematics. For efficiency, we had the robot associate multiple inputs with the same goal, collecting views of the goal from different perspectives. We also sampled from states that are unlikely to occur during a successful execution in order to promote recovery from errors. For example, tasks containing the “grasp” action primitive are trained with examples of inputs that are far from the final states associated with the “approach” action primitive. This enables the “grasp” action primitive to recover from a poor “approach” or changes due to a dynamic environment.
% Using grasping as an example, the keyframes would be signified as: initial pose, pregrasp pose, grasp, and lift.
%\jeremy{We should explicitly mention that the frames were collected asynchronously somewhere, and make it clear how we collected them in pairs. Maybe a nice diagram is the best solution.}
% In order to facilitate the reduction in size of the state space in a course-to-fine manner, we learn to map a set of plausible initial frames to a singular final frame.
% Although most works collect data for imitation learning sequentially, we decide to do so in an asynchronous manner, allowing for more efficient data collection.
This method allows our algorithm to be resilient to potentially imprecise predictions, thereby strengthening the robustness of the system. This is related to the concepts of funnels \cite{mason1985mechanics and pre-image backchaining \cite{lozano1984automatic} that have inspired recent work in robust feedback motion planning \cite{majumdar2017funnel}.}

% To expedite data collection, we developed a semi-autonomous method of generating initial keyframes. This method consisted of randomly perturbing the end-effector pose in tandem with a human teleoperating the robot \jeremy{omit? adds complexity, potentially confusing}.

To further enhance the efficiency of data collection, items relevant to other tasks were deliberately included in many initial frames. This strategy allows us to map identical input images to a final keyframe for each task relevant to the input image, consequently generating substantially more data points per image in the dataset. Moreover, this has the dual benefit of bolstering the robustness of text conditioning by exposing the network to negative examples.

Our data collection approach, therefore, not only enables a more streamlined and efficient process, but also exposes our algorithm to a diverse set of environments and object configurations. This data collection methodology was key to achieving the necessary robustness to generalize across a wide range of real-world tasks and environments. Conducted over the course of 30 hours, our data collection process yielded over 26,000 high-quality keyframe pairs, the equivalent of approximately 10,000 distinct task demonstrations.

\textbf{Comparing Our Data Collection Method to Sequential Demonstrations}

We estimate that we collected the equivalent of approximately 10,000 task demonstrations in 30 hours. In pilot experiments, we measured the time it takes to collect keyframes sequentially, coming up with a lower-bound estimate of 1 minute per demonstration. Assuming this value, collecting 10,000 task demonstrations would have taken approximately $10,000 / 60 = 167$ hours, as opposed to the 30 hours we dedicated to collecting data.

% \jeremy{30 hours, 23k unique images, 40k keyframe pairs, 26k keyframe pairs after filtering. We have 2.7 keyframe pairs per task, so this is equivalent to 9792 demonstrations. After testing, we found that it would take about 60 seconds to collect a single demonstration the traditional way. To get 9792 demonstrations in sequence, this would take 163 hours. We instead got the same amount of data in 30 hours = 5x faster}

% \jeremy{we should somehow be more clear about how data was collected, why it's efficient, and why it works. Most confusing part of the paper}

% \jeremy{Include nice visualization of all the initial and final camera poses for each step. Maybe just a single recording session for each pair of steps.}

\section{Details on Real-world Experiments}
\label{appendix:real-world-experiments}

The real-world experiments for \method{} are conducted in unseen environments and with held-out objects (Figure \ref{fig:train-test-side-by-side} and Table \ref{tab:test-definition}). The action primitive sequences are also unique to each task. For example, the ``pick up the apple" task shown in Figure \ref{fig:pick-up-apple-3d-pred} consists of \textit{``approach", ``grasp", and ``lift"} action primitives.

\begin{figure}[t]
  \centering
  % \vspace{2mm}
  \includegraphics[width=1\linewidth]{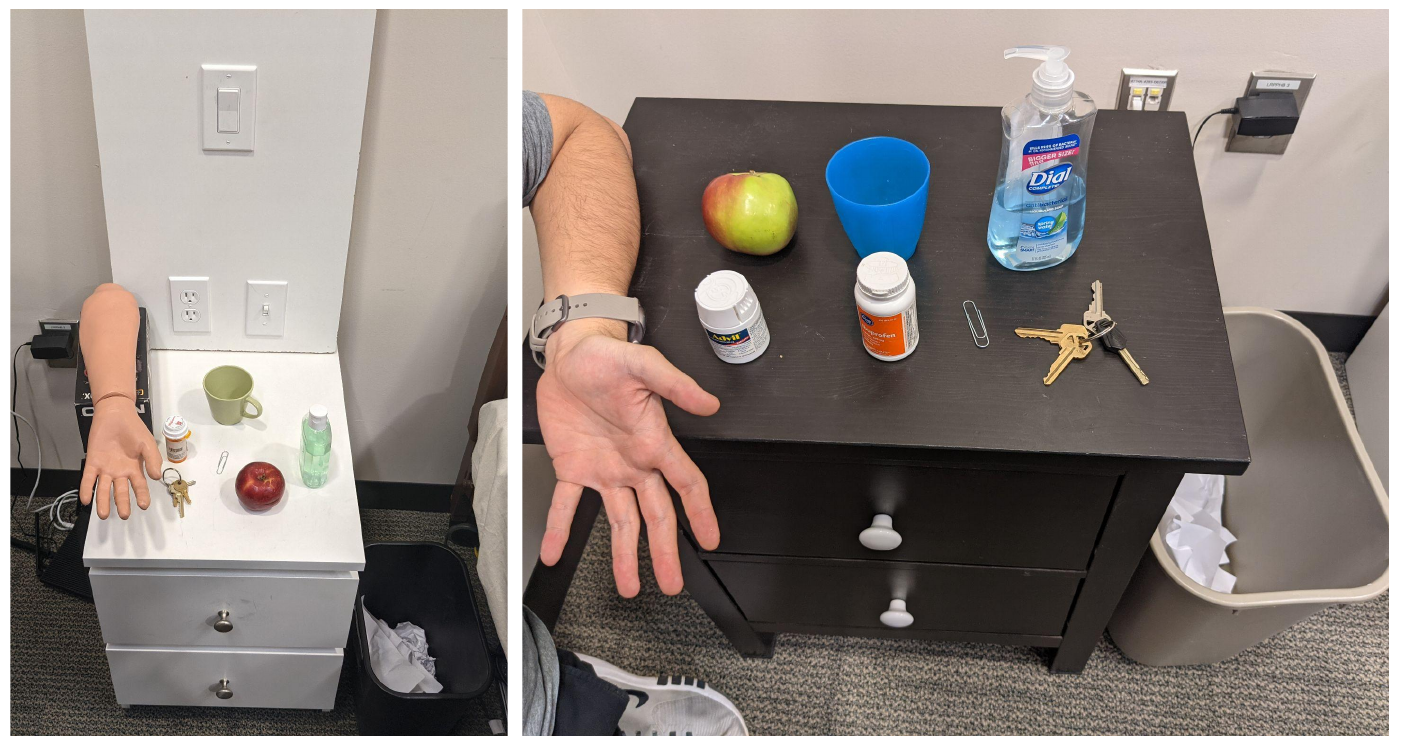}
  \vspace{-5mm}
  \caption{\textbf{Left:} Objects present in the training set. \textbf{Right:} Objects present in the test set and ablation studies. \cody{make it clear that the train set of object was different than the test!!!}}
  \label{fig:train-test-side-by-side}
   %\vspace{-15mm}
\end{figure}

\begin{figure}[t]
  \centering
  % \vspace{2mm}
  \includegraphics[width=1\linewidth]{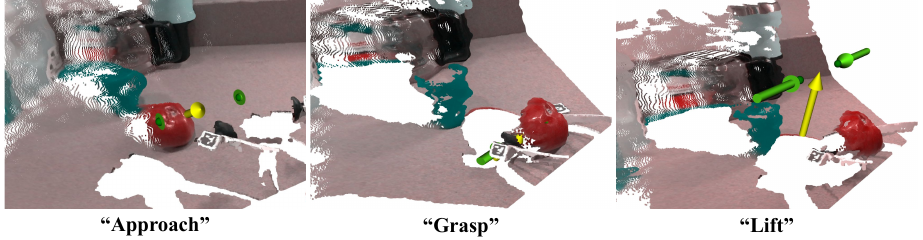}
  % \vspace{-2mm}
  \caption{Force objectives prediction in 3D perspective when conducting ``pick up the apple" task in a kitchen environment. Yellow arrow represents applied force $F_A$ and green arrows represent grip force $F_G$ acting on the target object.}
  \label{fig:pick-up-apple-3d-pred}
   %\vspace{-15mm}
\end{figure}

We run the model at 8 Hz, providing kinematic and force objectives for visual-force servoing. Through these experiments, we show that \method{} is able to perform well in scenarios with unseen objects and environments. 

% \begin{table*}
% \small 
% \centering
% \begin{tabular}{c|c|c|c}
%     \textbf{Task} & \textbf{Environment} & \textbf{Objects} & \textbf{Action Primitives}\\\hline
%     Pick up the apple & Kitchen & Apple, top drawer & Approach, Grasp, Lift  \\
%     Pick up the medicine bottle & Bedroom & Medicine bottle, top drawer & Approach, Grasp, Lift\\
%     Pick up the keys & Bedroom & Keys, top drawer & Approach, Grasp, Lift\\
%     Pick up the paperclip & Bedroom & Paperclip, top drawer & Approach, Grasp, Lift\\
%     Pick up the hand sanitizer & Kitchen & Hand sanitizer, counter top & Approach, Grasp, Lift \\
%     Pick up the cup & Kitchen & Cup, counter top & Approach, Grasp, Lift\\
%     Place object in the trash & Bedroom  & Medicine bottle, trash bin & Approach, Ungrasp\\
%     Place object in the hand & Bedroom & Medicine bottle, real human hand & Approach, Ungrasp\\
%     Turn off the light switch & Atrium & Light switch & Approach, Push \\
%     Open the drawer & Bedroom  & Bedside drawer & Approach, Grasp, Pull\\
% \end{tabular}
% \caption{Tasks, environments, objects and success metrics \jeremy{Fit this into single column and insert into main paper}}
% \label{tab:test-definition}
% \vspace{-5mm}
% \end{table*}

\begin{table*}
\centering
\small
\begin{tabular}{c|c|c|c|c}
    & \textbf{Overall Task Success} & \textbf{Subgoal 1} & \textbf{Subgoal 2} & \textbf{Subgoal 3}\\\hline
    \network{} (Ours) & 81\//100 (81\%) & 96\//100 (96\%) & 93\//96 (97\%) & 54\//65 (83\%) \\\hline
    w/o forces & 10\//20 (50\%) & 13\//20 (65\%)  & 11\//13 (85\%) & 6\//7 (86\%) \\\hline
    w/o augmentation & 5\//20 (25\%) & 11\//20 (55\%) & 7\//11 (64\%) & 5\//7 (71\%) \\ \hline
    w/o depth & 4\//20 20\%) & 8\//20 (40\%) & 6\//8 (75\%) & 3\//3 (100\%) \\\hline 
    w/o pre-training & 4\//20 (20\%) & 5\//20 (25\%) & 4\//5 (80\%) & 3\//3 (100\%) \\\hline 
    w/o text conditioning & 0\//20 (0\%) & 9\//20 (45\%) & 0\//9 (0\%) & - \\\hline 
\end{tabular}
\vspace{3mm}
\caption{Detailed task success rate for ForceSight ablation on real-world experiments. \jeremy{Omit from paper.}}
\label{tab:detailed-task-ablations}
\end{table*}

From the analysis presented in Table \ref{tab:detailed-task-ablations}, it is evident that \method{} outperforms other approaches in terms of task success rate. Specifically, when the low-level controller disregards the force goals, both \textit{subgoal 1} and \textit{subgoal 2} exhibit lower success rates. This can be attributed to the robot's inability to accurately approach and grip the target object. For example, the gripper will prematurely grasp the drawer's handle without applying force to the drawer during the approach stage. Additionally, the absence of data augmentation adversely affects the model's ability to perceive new objects, as evidenced by its struggles in recognizing unseen objects such as the green apple and the black drawer. By excluding depth information from the model, the success rate of \textit{subgoal 1} decreases, primarily because this stage (``approach" action) heavily relies on accurate depth perception. Moreover, pre-training proves to be a valuable technique for enabling the robot to learn with minimal data. When our ViT was initialized with random weights rather than pre-trained weights, the affordance map prediction was worsened, resulting in a lower success rate with the same training configurations. Interestingly, when text conditioning is removed, the model can successfully detect interesting objects as goals (9 out of 20 in \textit{subgoal 1}), but fails to determine the appropriate actions to perform with the target object, seen in \textit{subgoal 2}.

\begin{figure}[H]
  \centering
  % \vspace{2mm}
  \includegraphics[width=1\linewidth]{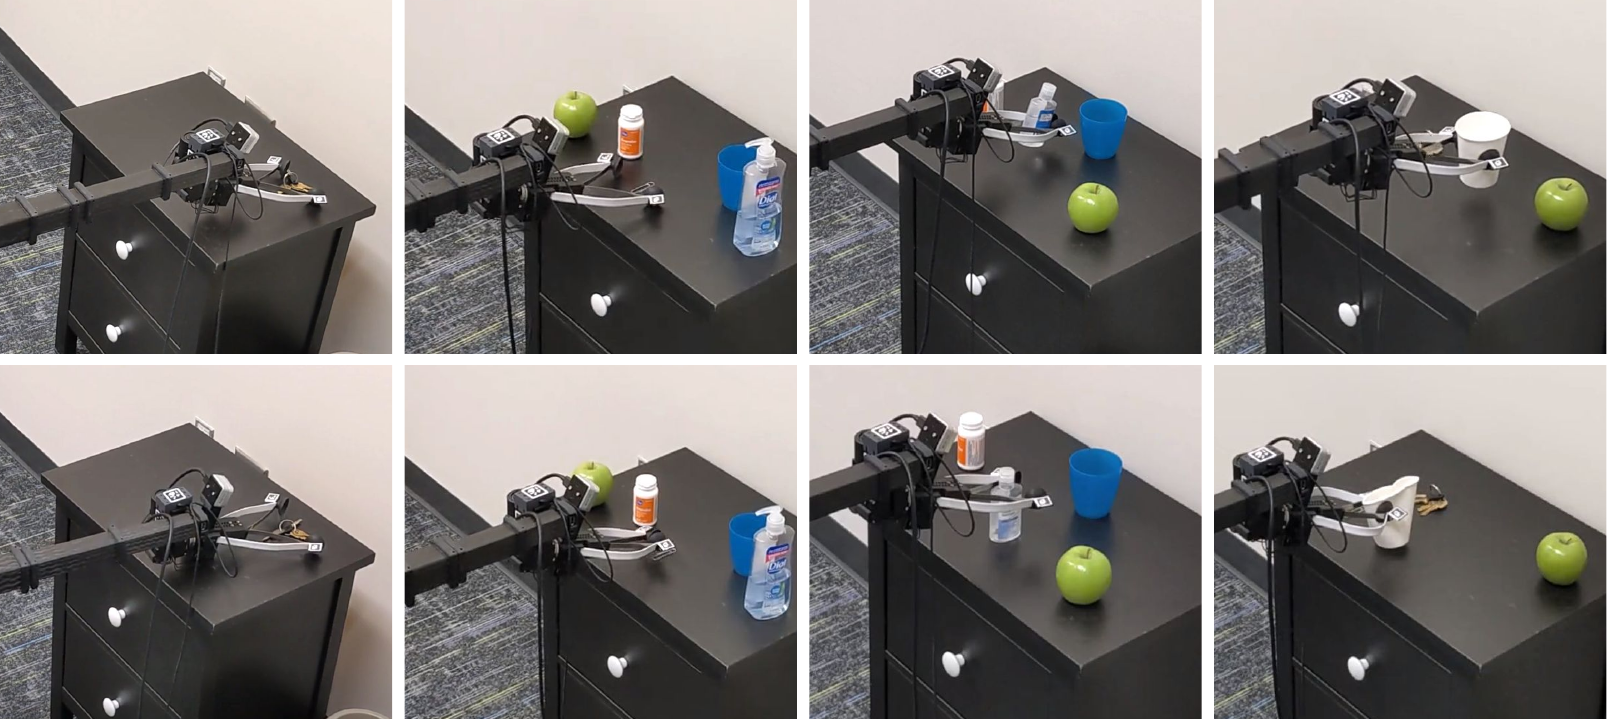}
  % \vspace{-2mm}
  \caption{\method{} with force goals (top) vs. \method{} without force goals (bottom). Comparison videos are shown on the \href{https://force-sight.github.io/}{website}.}
  \label{fig:no-force-failures}
   %\vspace{-15mm}
\end{figure}

% w/o force 4/6 success for 1-2 subgoals, 8/9 success for 1-3 subgoals for a total of 12/20

\begin{table}[H]
\centering
\scriptsize
\begin{tabular}{c|c|c|c|c}
    & \textbf{Overall} &  \textbf{Subgoal 1} & \textbf{Subgoal 2} & \textbf{Subgoal 3} \\
    & \textbf{Task Success} & & &\\\hline
    \textbf{w/ forces (\method{})} & \textbf{18/20 (90\%)} & \textbf{95\%}  & \textbf{90\%} & \textbf{76\%} \\
\hline
    w/o forces & 45\% & 80\% & 45\% & 29\% \\ 
    % w/ binary force & 80\%  & 100\% & 90\% & 59\% \\ 
\end{tabular}
\caption{Detailed evaluation of task success rate v.s. presence of force as an input modality to the low-level controller.  \jeremy{not sure whether to include binary grip or not} \cody{make the 90 percent vs 40 percent more prominent}}
\label{tab:detailed-force-ablations}
\end{table}

\youliang{move this to above}

In Table \ref{tab:detailed-force-ablations}, we present a comprehensive ablation study centered on the employment of force. In general, using force as a modality leads to generally improved task performance, especially in tasks that require tactile sensitivity, such as picking up a paperclip. When the controller does not consider force, the number of errors and misjudgments increases, especially when handling delicate tasks. The robot often exerted too much force on the object, or the gripper failed to grip. Tasks such as "place object in the trash" were not affected since they involve less tactile interactions with the surroundings.

% \jeremy{TODO: add CLIP and Dino v2 experiments}
% \jeremy{TODO: mention LLM and learning from human video}
% \jeremy{TODO: add pictures of objects and unseen instances. also add pictures of environments}

\youliang{Emergent Properties moved to top}
% \section{Emergent Properties}
% \label{appendix:emergent-properties}

% After training, we observed multiple surprising behaviors exhibited by \network{}. Notably, \network{} demonstrated a surprising flexibility and adaptability in its treatment of action primitives in relation to various objects. For instance, \network{} managed to apply certain action primitives to objects without any explicit representation of such actions during the training phase. For example, if given the action primitive ``grasp" in combination with a prompt concerning a light switch or the action primitive ``push" in combination with a prompt concerning a medicine bottle, the model responded with predictions corresponding to the specified actions, despite these specific actions being absent in the training data. Emergent properties are shown in Figure \ref{fig:agent-agnostic} and \ref{fig:multistep-pred}.

% We also observe that \network{} is agnostic to the gripper it is observing; although during training we only show the network a single gripper, it learns to completely ignore the visual features associated with the gripper, and the predictions were observed to be invariant to the type of gripper the RGBD camera was mounted to, and even works without any gripper present in the field of view.

\section{Determining Output Representation}
\label{appendix:output-rep}

% \vspace{-28mm}

We experimented with three output representations of the fingertip locations, namely: Regression-based, Pixel-Space Contact points, and Pixel-Space Centroid output representation.

The regression-based representation directly minimizes the $L_1$ error of the contact point locations. We observed this representation to work well in simplified environments with a single object, but it struggled in situations where there were multiple plausible contact points, especially when two semantically relevant objects were present in the input image. We hypothesize that this is because the $L_1$ objective encourages the model to find the mean of the target distribution of plausible fingertip locations. In this situation where this distribution is multimodal, the model produces estimates that average out the different modes of the distribution, resulting in a model that provides suboptimal predictions for all modes.

\begin{table*}
\centering
\small
% \vspace{-10mm}
% \vspace{-10mm}
\begin{tabular}{c|c}
    \textbf{Representation} & \textbf{Avg. Fingertip Dist (m)}\\\hline
    % Perceiver-Actor & 0\%  \\\hline
    % Cliport & 0\%  \\\hline
    Contact point regression & 0.429 \\\hline
    Contact point classification (cls.) & 0.107 \\\hline
    Centroid cls. + gripper width + yaw & 0.057 \\\hline
    Centroid cls. + gripper width + yaw + Action Primitive &  \textbf{0.036} \\\hline
\end{tabular}

\caption{Representation Ablations.}
\label{tab:rep-ablations}
% \vspace{3mm}
\vspace{-3mm}
\end{table*}

To tackle this issue of estimating 3D locations in a multimodal distribution, we instead formulated our optimization as a classification problem. To additionally take advantage of the knowledge present in our pre-trained ViT, we decouple the representation into pixel-wise classification and depth-wise regression. This has the additional benefit of highly interpretable predictions, as the affordance map is a distribution that may be overlayed on the input image. We initially treated contact points individually, but found that locations associated with the left and right fingertip didn't necessarily correspond to one another, often leading to physically implausible predictions due to the lack of correspondence between fingertip locations.

To address this correspondence issue, we reparameterized our representations to instead classify the pixel location associated with the center of the contact points $C_{xy}$, perform regression on the depth estimates $C_z$ associated with the pixel location, and additionally predict the gripper width and the yaw $\psi$ so that the individual fingertip locations could be derived. The ablation of the output representation is shown in Table \ref{tab:rep-ablations}. A point to note that our current model does not factor in roll and pitch -- we have opted to keep roll and pitch constant in our method. That said, roll and pitch can be easily included by adding additional MLP heads.

The ForceSight system architecture comprises several components that work together to accomplish a text-conditioned task. It begins with a High-level Task Planner, which takes a text input and generates a sequence of action primitives representing subgoals. These action primitives, along with the RGBD input, are then passed to the ForceSight transformer model.

The ForceSight model processes the input and produces force-based objectives. These objectives are subsequently fed into the low-level controller, which generates joint motion commands for the robot to execute the task and its action primitive. This is done by using visual-servo control.

To determine when to switch to the next action primitive, the low-level controller compares the error between the current states and visual-force goals with a predefined threshold. If the error is below the threshold, the low-level controller initiates the switch to the next action primitive.

This entire process loop operates at a frequency of 8 Hz, allowing for multiple iterations until the task is completed successfully.

\section{Low-Level Controller}
\label{appendix:controller}
Our low-level controller receives 3D target contact and force goals located in the camera frame from \network{} and executes an action after each image frame observation in order to achieve these goals. Using an eye-in-hand camera, the low-level controller uses visual-force servoing to move the gripper closer to the visual-force goal. This approach reduces relative error and is insensitive to global calibration.

In our low-level control framework, we divide operations into two main components: Translation Control and Gripper Control.

\subsubsection{End-Effector Control: Minimizing Euclidean Translation, $\mathcal{E}_{\text{translation}}$ and Applied Force Error, $\mathcal{E}_{\text{applied force}}$}
Our aim here is to minimize both the Euclidean translation and the applied force error along the $XYZ$ axis:

\begin{equation}
\begin{split}
\mathcal{E}_{\text{translation}} &= || C_{\text{predicted}} - C_{\text{current}} ||_2 \\
\mathcal{E}_{\text{yaw}} &= || \psi_{\text{predicted}} - \psi_{\text{current}} ||_2 \\
\mathcal{E}_{\text{applied force}} &= || F_{\text{applied, predicted}} - F_{\text{applied, current}} ||_2
\end{split}
\end{equation}

Where $C_\textit{current} \in \mathbb{R}^{3}$ is the current translation of the fingertip centroid; $C_\textit{predicted} \in \mathbb{R}^{3}$ is the predicted translation of the fingertip centroid; $F_\textit{applied, current} \in \mathbb{R}^{3}$ is vector of the current applied force; $F_\textit{predicted} \in \mathbb{R}^{3}$ is the vector of the predicted applied force.

\subsubsection{Grasping Control: Minimizing Gripper Width, $\mathcal{E}_{\text{width}}$ and Grip Force Error, $\mathcal{E}_{\text{grip force}}$}
 For this objective, the goal is to minimize discrepancies in the gripper width and grip force, expressed as:
 
\begin{equation}
\begin{split}
\mathcal{E}_{\text{width}} &= || W_{\text{predicted}} - W_{\text{current}} ||_2 \\
\mathcal{E}_{\text{grip force}} &= || F_{\text{grip, predicted}} - F_{\text{ grip, current}} ||_2
\end{split}
\end{equation}

Where $W_\textit{current} \in \mathbb{R}$ is the current gripper width; $W_\textit{predicted} \in \mathbb{R}$ is the predicted gripper width; $F_\textit{grip, current} \in \mathbb{R}$ is the current grip force; $F_\textit{grip, predicted} \in \mathbb{R}$ is the predicted grip force.

The goal is to minimize the kinematic and force error in all directions in a step-wise manner. To better incorporate both kinematic and force modalities into the movement error,  we define a joint objective combining both errors. This is expressed as a movement control  $M_\text{end-effector} \in \mathbb{R}^3$ and $M_\text{gripper} \in \mathbb{R}$ in cartesian space, and then is executed by the controller in a step-wise manner.

\begin{equation}
\begin{split}
M_{\text{end-effector}} &= \mathcal{E}_{\text{translation}} + \lambda_\text{applied} \mathcal{E}_{\text{applied force}} \\
M_{\text{gripper}} &= \mathcal{E}_{\text{width}} + \lambda_\text{grip} \mathcal{E}_{\text{grip force}}\\
\end{split}
\end{equation}

The movement value determines the necessary movement that the robot should execute in order to reach the predicted objectives. By combining both kinematic and force objectives, the task can be executed more delicately, leading to improved performance. This approach is particularly useful in determining whether the current action primitive has been successfully completed, and whether the next action primitive should be passed as an input to \network{}. Results are shown in Table \ref{tab:ablations}.

We recognize that there are many options for implementing the low-level controller; for example, our policy can easily be substituted for a goal-conditioned reinforcement learning policy \cite{liu2022goal}. We could also plausibly replace the F/T sensor with a system that estimates these values from motor current or from vision \cite{collins2022force, collins2023visual}.

\section{Training Details}
\label{appendix:training}

We train \network{} for 20 epochs using the Adam optimizer \cite{kingma2014adam}, corresponding to a total of 500,000 iterations. Our training procedure processes 224x224 RGBD images in batches of eight with a learning rate of 5e-5. 

\network{}'s loss function is as follows:
\begin{align}
L_{A} &= -\sum_{i,j=0}^{H, W}(\beta * A log(\hat{A}) + (1 - A) log(1 - \hat{A})) \label{eq:L_A} \\
L_{D} &= A * ||D - \hat{D}||_1 \label{eq:L_D} \\
L_{F_A} &= ||F_A - \hat{F_A}||_2 \label{eq:L_F} \\
L_{F_G} &= ||F_G - \hat{F_G}||_2 \label{eq:L_G} \\
L_{W} &= ||W - \hat{W}||_2 \label{eq:L_W} \\
L_{\psi} &= ||\psi - \hat{\psi}||_2 \label{eq:L_psi} \\
\end{align}

Where $L_A$ is the affordance map cross-entropy loss, $L_D$ is the masked depth map MAE loss, $L_{F_A}$ is the MSE of applied force, $L_{F_G}$ is the MSE of grip force, $L_W$ is the MSE for gripper width, and $L_{\psi}$ is the MSE for yaw.

\network{} is trained with the weighted sum of the individual losses:
\begin{align}
L = \sum_{i \in \{A, D, F_A, F_G, W, \psi\}} \lambda_i L_i
\label{eq:L}
\end{align}

Balancing the impact of distinct loss components, we assign coefficients as follows: $\lambda_A = 1, \lambda_D = 5e4, \lambda_{F_A} = 0.2, \lambda_{F_G} = 0.2, \lambda_W = 0.2$, and $\lambda_{\psi} = 0.2$. In our weighted cross-entropy loss associated with affordance map prediction (Equation \ref{eq:L_A}), we place a stronger emphasis on the correct localization of contact points by assigning a $\beta$ value of 100, emphasizing the importance of correctly identifying locations of interest.

Our ground truths for pixel-wise classification take the form of multi-hot encodings, where circles with a radius of 10 pixels pinpoint the tool center point's coordinates. We found that this denser representation of the ground truth produced rich heatmaps while maintaining good performance.

To further improve the robustness of our model and encourage generalization, we apply brightness, saturation, contrast, and hue augmentation to the RGB channels of the input.

We also include a data filtering step that excludes examples where the ground truth lies outside the camera's field of view. This process minimizes potential inaccuracies that could arise from attempting to predict beyond the field of view.

Additionally, we find that appending action primitives to the text prompts enhances the model's performance. This strategy clearly defines the boundaries between keyframes, enhance the transitions between subgoals. (Table \ref{tab:rep-ablations}).

\section{Using Large Language Models to Assign Action Primitives}
\label{appendix:llm}
\begin{figure}[H] % 'H' specifier forces the figure to be placed here
  \centering
  % \vspace{2mm}
  \includegraphics[width=.6\linewidth]{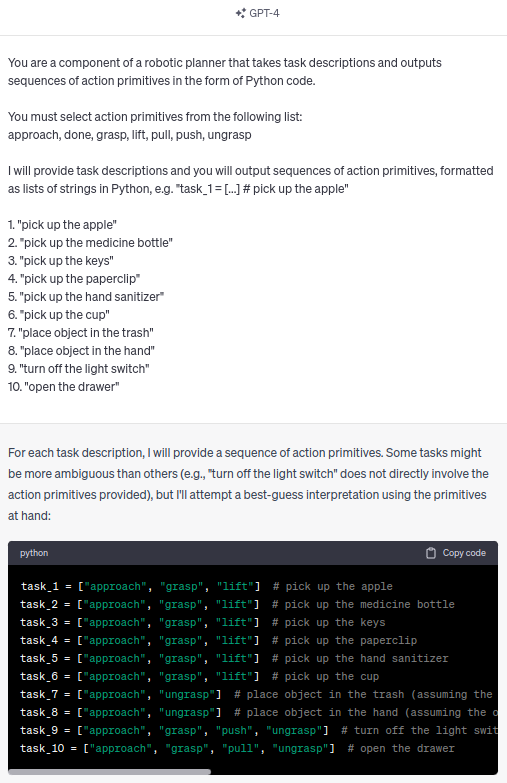}
  % \vspace{-2mm}
  \caption{We demonstrate how a large language model (GPT-4) could plausibly be used to assign action primitives to task descriptions.}
  \label{fig:gpt4_output}
   \vspace{-5mm}
\end{figure}

In place of the finite state machine that determines which action primitive will be appended to the input prompt, we hypothesize that a large language model could assign action primitives to unseen prompts. We support this hypothesis by prompting GPT-4, a large language model, to perform this operation, and observe promising initial results (Figure \ref{fig:gpt4_output}).
